# Supplementary material for: Data-driven memory-dependent abstractions of dynamical systems
Source: arXiv:2212.01926 source file (2022-12-04)
Supplement: Supplementary file 1 [file Discussion_Murak_paper.tex]

\section{Discussion about the paper \cite{DSA:21}}

Raphael sent us an email on the 16th of October, 2022, raising some technical questions about paper \cite{DSA:21}. Below we will try to briefly summarise their results, as this will serve as a starting point for a more technical discussion. In doing so, we will be using a slightly different mathematical notation.

The main message of the paper is to define an approximate alternating simulation notion between continuous-time dynamical systems and discrete-state ones and show that such a notion is adequate to perform verification of bounded temporal specifications. Then, the authors present a sampling mechanism that can be used to obtain a pair of models that satisfies the developed notion of alternating simulation. 

While reasoning about their results, we decided to use the following mathematical notation:

\begin{itemize}
    \item $\mathcal{S}$ represents a set of discrete states. An element of $\mathcal{S}$ will be denoted by $s$ and its cardinality will be denoted by $n_s$.
    \item $\mathcal{A}$ represents a set of discrete actions. An element of $\mathcal{A}$ will be denoted by $a$ and its cardinality by $n_a$.
    \item $\mathcal{X}$ represents a continuous state-space. An element of $\mathcal{X}$ will be denoted by $x$ and its dimension by $n_x$.
    \item $\mathcal{U}$ represents the set of continuous actions. An element of $\mathcal{U}$ will be denoted by $u$ and its dimension by $n_u$.
\end{itemize}

Considering the notation above, we would like to relate the behavior of two dynamics: one that evolves in a continuous space and another that evolves in a discrete one. Assume that the continuous dynamics is defined by 
\begin{equation}
    x_+ = f(x,u), \quad x(0) = x_0
    \label{eq:ContinuousDynamics}
\end{equation}
where $x_0$ is a given initial condition, and the notation $x_+ = f(x,u)$ indicates that the next state $x_+$ is generated from the previous state $x$ and input $u$ by applying the map $f:\mathcal{X} \times \mathcal{U} \mapsto \mathcal{X}$. To relate \eqref{eq:ContinuousDynamics} to a discrete dynamic we use a mapping (not necessarily single-valued) $\phi_{\mathcal{X}}: \mathcal{X} \mapsto \mathcal{S}$ that relates the state space of both dynamics, and another mapping $\phi_{\mathcal{U}}: \mathcal{X} \times \mathcal{U} \mapsto \mathcal{A}$ that relates the corresponding input spaces.

\begin{assumption}
    We assume that the mapping $\phi_{\mathcal{X}}$ is such that\footnote{I was planning to draw the corresponding commutative diagram, but thought this would take a bit of time to do it.} $\phi = \bar{\phi} \circ \pi$, where $\pi$ is the quotient mapping (due to the partition of the state space $\mathcal{X}$) and $\bar{\phi}$ is some mapping between the quotient space $\frac{\mathcal{X}}{\sim}$ and $\mathcal{S}$.
\end{assumption}

Notice that if $\bar{\phi}$ is an one-to-one mapping we can identify the states in $\mathcal{S}$ with each partition element of the continuous space $\mathcal{X}$. As we would like to use the discrete model $(\mathcal{S},\mathcal{A})$ to assert properties of the original model $(\mathcal{X},\mathcal{U})$, it is reasonable to impose the following restrictions on $\phi_\mathcal{X}$ and $\phi_{\mathcal{U}}$:

\begin{itemize}
    \item Let $\mathcal{S}_0$ be the possible initial states of $\mathcal{S}$ and $\mathcal{X}_0$ be a region of the continuous state space from which we initialise the dynamics \eqref{eq:ContinuousDynamics}. Then, it is intuitive to require that $\phi_{\mathcal{X}}(\mathcal{X}_0) = S_0$, i.e., every element in $\mathcal{X}_0$ is mapped into an element of $S_0$, and conversely.

    \item For every possible transition in the discrete-space, there corresponds an admissible state-input pair whose next state is in the inverse image under the mapping $\phi_{\mathcal{X}}$ for the associated next state in the discrete-space. This is the sort of condition that is simpler and cleaner to explain using maths. We require that
    \[
        \forall (s,a) \in \mathcal{S} \times \mathcal{A}, \exists (x,u) \in \mathcal{X} \times \mathcal{U} \in (\phi_{\mathcal{X}}^{-1}(y) \times \mathbb{R}^{n_u}) \cap \phi^{-1}_{\mathcal{U}}(a) \text{ such that } f(x,u) \in \phi_{\mathcal{X}}^{-1}(T(s,a)),
    \]
    where $T: \mathcal{S} \times \mathcal{A} \mapsto \mathcal{S}$ is the transition mapping describing the discrete dynamics.
\end{itemize}

One can argue that the above description coincides with the standard notion of alternating simulation relation that has been developed in the symbolic control literature. The authors in \cite{DSA:21} propose a modification of the second bullet point above that may be adequate to generate abstraction of black box models. Before we introduce such a modification, let's define a collection of mathematical notation.

\begin{itemize}
    \item In parallel to \eqref{eq:ContinuousDynamics}, the discrete dynamics will evolve as 
    \begin{equation}
        s_+ = T(s,a), \quad s(0) = s_0.
        \label{eq:DiscreteDynamics}
    \end{equation}
    \item Elements of $\mathcal{S}$ will be denoted by $s_i,~i = 1, \ldots, n_s$; elements of $\mathcal{A}$ by $a_j,~j = 1, \ldots, n_u$; and elements of the quotient space either by  $\bar{x}_\ell,~\ell = 1, \ldots, p$, or by $P_\ell$, where the latter notation emphasizes that we are referring to a specific element of the partition.  

    \item The authors in \cite{DSA:21} aim at defining the mappings $\phi_{\mathcal{X}}$ and $\phi_{\mathcal{U}}$ through a sampling procedure, and hence we need to define a few quantities. For each element $P_\ell$, we define a collection o probabilities measure whose support is $P_\ell$, for instance, a uniform distribution with desired support. In fact, let's denote by $\mathbb{P}_\ell$ the uniform probability with support equal to\footnote{I am being a bit sloppy here, as I am not being careful with closedness issues. We can fix that later.} $P_\ell$ and, for a fix $\epsilon \in (0,1)$ and $u \in \mathcal{U}$, define the set
    \[
        \mathcal{S}^m \supset A_\ell(\epsilon,u) = \{ \bar{y} = (y_1,\ldots,y_m) \in P_\ell^m: V(\mathcal{H}_m(\bar{y},u) )\leq \epsilon \}, 
    \]
    where 
    \[
        \mathcal{H}_m(\bar{y},u) = \{ y \in \mathcal{P}_\ell: f(y,u) \in \cup_{r = 1}^{|T(s,a)|} \phi_{\mathcal{X}}^{-1} (s_+^r), \quad s_+^r \in T(s,a), \quad s = \phi_{\mathcal{X}}(y_i),~i = 1, \ldots, m, a = \phi_{\mathcal{U}}(u)   \}
    \]
    represents the points in the element of the partition $P_\ell$ for which the next state under action $u$ belongs to $\cup_{r = 1}^{|T(s,a)|} \phi_{\mathcal{X}}^{-1} (s_+^r)$, where $s_+^r$ is any possible next state of the discrete model $(\mathcal{S},\mathcal{A})$ from the state-action pair $(s,a)$, and where
    \[
        V(\mathcal{H}_m(\bar{y},u)) = \mathbb{P}_\ell \{ \mathcal{H}_m(\bar{y},u) \}.
    \]

    \item We are now in position to state equation (4) of \cite{DSA:21} using the notation we have presented so far and therefore understand their PAC notion of alternating simulation between two systems. Indeed, they say that system $(S,\mathcal{A})$ is an $(\epsilon,\beta)$-PAC alternating simulation of\footnote{I am not considering the approximate definition as they are considering the paper} $(\mathcal{X},\mathcal{U})$ if the second bullet point above is replaced by
        \begin{itemize}
            \item $\forall (s,a) \in (\mathcal{S},\mathcal{A}),~\exists (x,u) \in (\phi_{\mathcal{X}}^{-1}(y) \times \mathbb{R}^{n_u}) \cap \phi^{-1}_{\mathcal{U}}(a)$ such that for some $m \in \mathbb{N}$ we have that, for all $\ell = 1, \ldots, p,$
            \[
                \mathbb{P}_\ell^m \{ A_{\ell}(\epsilon,u) \} \geq 1 - \beta.
            \]
        \end{itemize}
    Or, in other words, there exists a finite number of samples for which, with confidence larger than $1-\beta$, the probability that the next state of the continuous dynamics is contained in the partitions induced by such samples is larger than $1-\epsilon$.
\end{itemize}

With the above notions of PAC-alternating simulation relation, the authors of \cite{DSA:21} then claim that this is enough to verify bounded temporal logical properties and Raphael made the following comment: ``My problem is with Eq. $(7)$ in Thm $1$: they say they ``iterate $m$ times 
condition $(iii)$ in Definition $4$''. More precisely, they decompose the 
event $(x_{1,1},...,x_{1,m})$ (the trajectory in the concrete system) into 
m events, and then they say that the probability of $(x_{1,1},...,x_{1,m})$ 
is the product of the probabilities of the elementary events. This is 
just not correct: The concrete system is a deterministic system; thus, 
$x_{1,i}$ is a deterministic function of $x_{1,i-1}$, there is no sampling 
anymore at step i!''

We will now reason about the comment Raphael made above. To this end, let me restate their theorem using the notation we have introduced in this section.

\begin{theorem}
    Let $(\mathcal{X},\mathcal{U})$ be a continuous-time dynamics evolving according to \eqref{eq:ContinuousDynamics} and $\varphi$ be a bounded specification of size $N$. Assume that a discrete-time dynamics as in \eqref{eq:DiscreteDynamics} is a $(\epsilon,\beta)$-PAC alternating simulation of \eqref{eq:ContinuousDynamics}. If there exists a control law $K_d: \mathcal{A} \times \mathbb{N} \mapsto \mathcal{S} $ such that the closed-loop system $(\mathcal{S},\mathcal{A},K_d) \models \varphi$, then there exists a control law $K_c: \mathcal{X} \times \mathbb{N} \mapsto \mathcal{X}$ such that, for all $k \leq N$, with confidence at least $1-\delta$, we have ``The probability that the closed-loop system $(\mathcal{X},\mathcal{U},K_c)$ satisfies $\varphi$ in the first $k$ steps is at least larger than $(1-\epsilon)^k$.''
    \label{theo:DAS_theo1}
\end{theorem}

Below are few comments:

\begin{itemize}
    \item I agree with Raphael. The notion of $PAC$-alternating simulation defined in the paper is based on the fact that we are able to sample (uniformly) at each element of the partition of the state space $\mathcal{X}$. Well, if you sample the initial state uniformly, I believe that (assuming such a simulation between the models) one can make their argument hold in the first step. However, and as Raphael suggested in his comment, how would you bound the quantity $\mathbb{P}_{\phi_{X}(x_1)} \{ f(x_1,u_1) \in \cup_{r = 1}^{|T(s_1,a_1)|} \phi_{\mathcal{X}}(s_+R)  \}$ if $x_1$ is not uniformly sampled from its corresponding partition but actually the image of a point that has been uniformly sampled from the partition of $x_0$ and then following a deterministic dynamics?
\end{itemize}

\subsection{A counterexample for the abstraction results in \cite{DSA:21}}

Unless I am missing something, I think I have found a very weird dynamical system for which the procedure in \cite{DSA:21} will fail. I will describe the example in words here, but my plan is to go to the whiteboard tomorrow and explain my reasoning to you. 

Let $P_0,P_1,P_2,P_3,P_4, P_5$ be an arbitrary partition of the state space, with labels given by $\alpha,\alpha,\alpha,\beta,\alpha,\beta$, respectively. Assume that we have two possible  actions at each partition, represented by $a$ and $b$. Applying action $a$ at the initial partition leads us to partitions $P_1, P_2$ with probability $1-\epsilon$ and to partition $P_3$ with probability $\epsilon$ (these probabilities come from the fact that we are sampling the initial partition uniformly), while applying action $b$ at $P_0$ leads always to partitions $P_1,P_2$. Observe that $P_1,P_2$ have both label $\alpha$, while $P_3$ has label $\beta$. \textit{Assume the dynamics under study is such that the image of $P_0$ under action $b$ is a segment (that is, its affine hull is a one-dimensional space) that has non-empty intersection with $P_1$ and $P_2$. Assume also that the image of this segment under both actions leads to partition $P_5$, while the set $P_1 \cup P_2 \setminus \{ \text{ segment } \}$ under action $b$ leads to $P_4$. $P_4$ and $P_5$ will be deadlock states for both actions}.  As the number of samples goes to infinity, the non-deterministic abstraction that one would generate is the following:

\begin{figure}[h]
    \centering
    \includegraphics[width = 0.7\columnwidth]{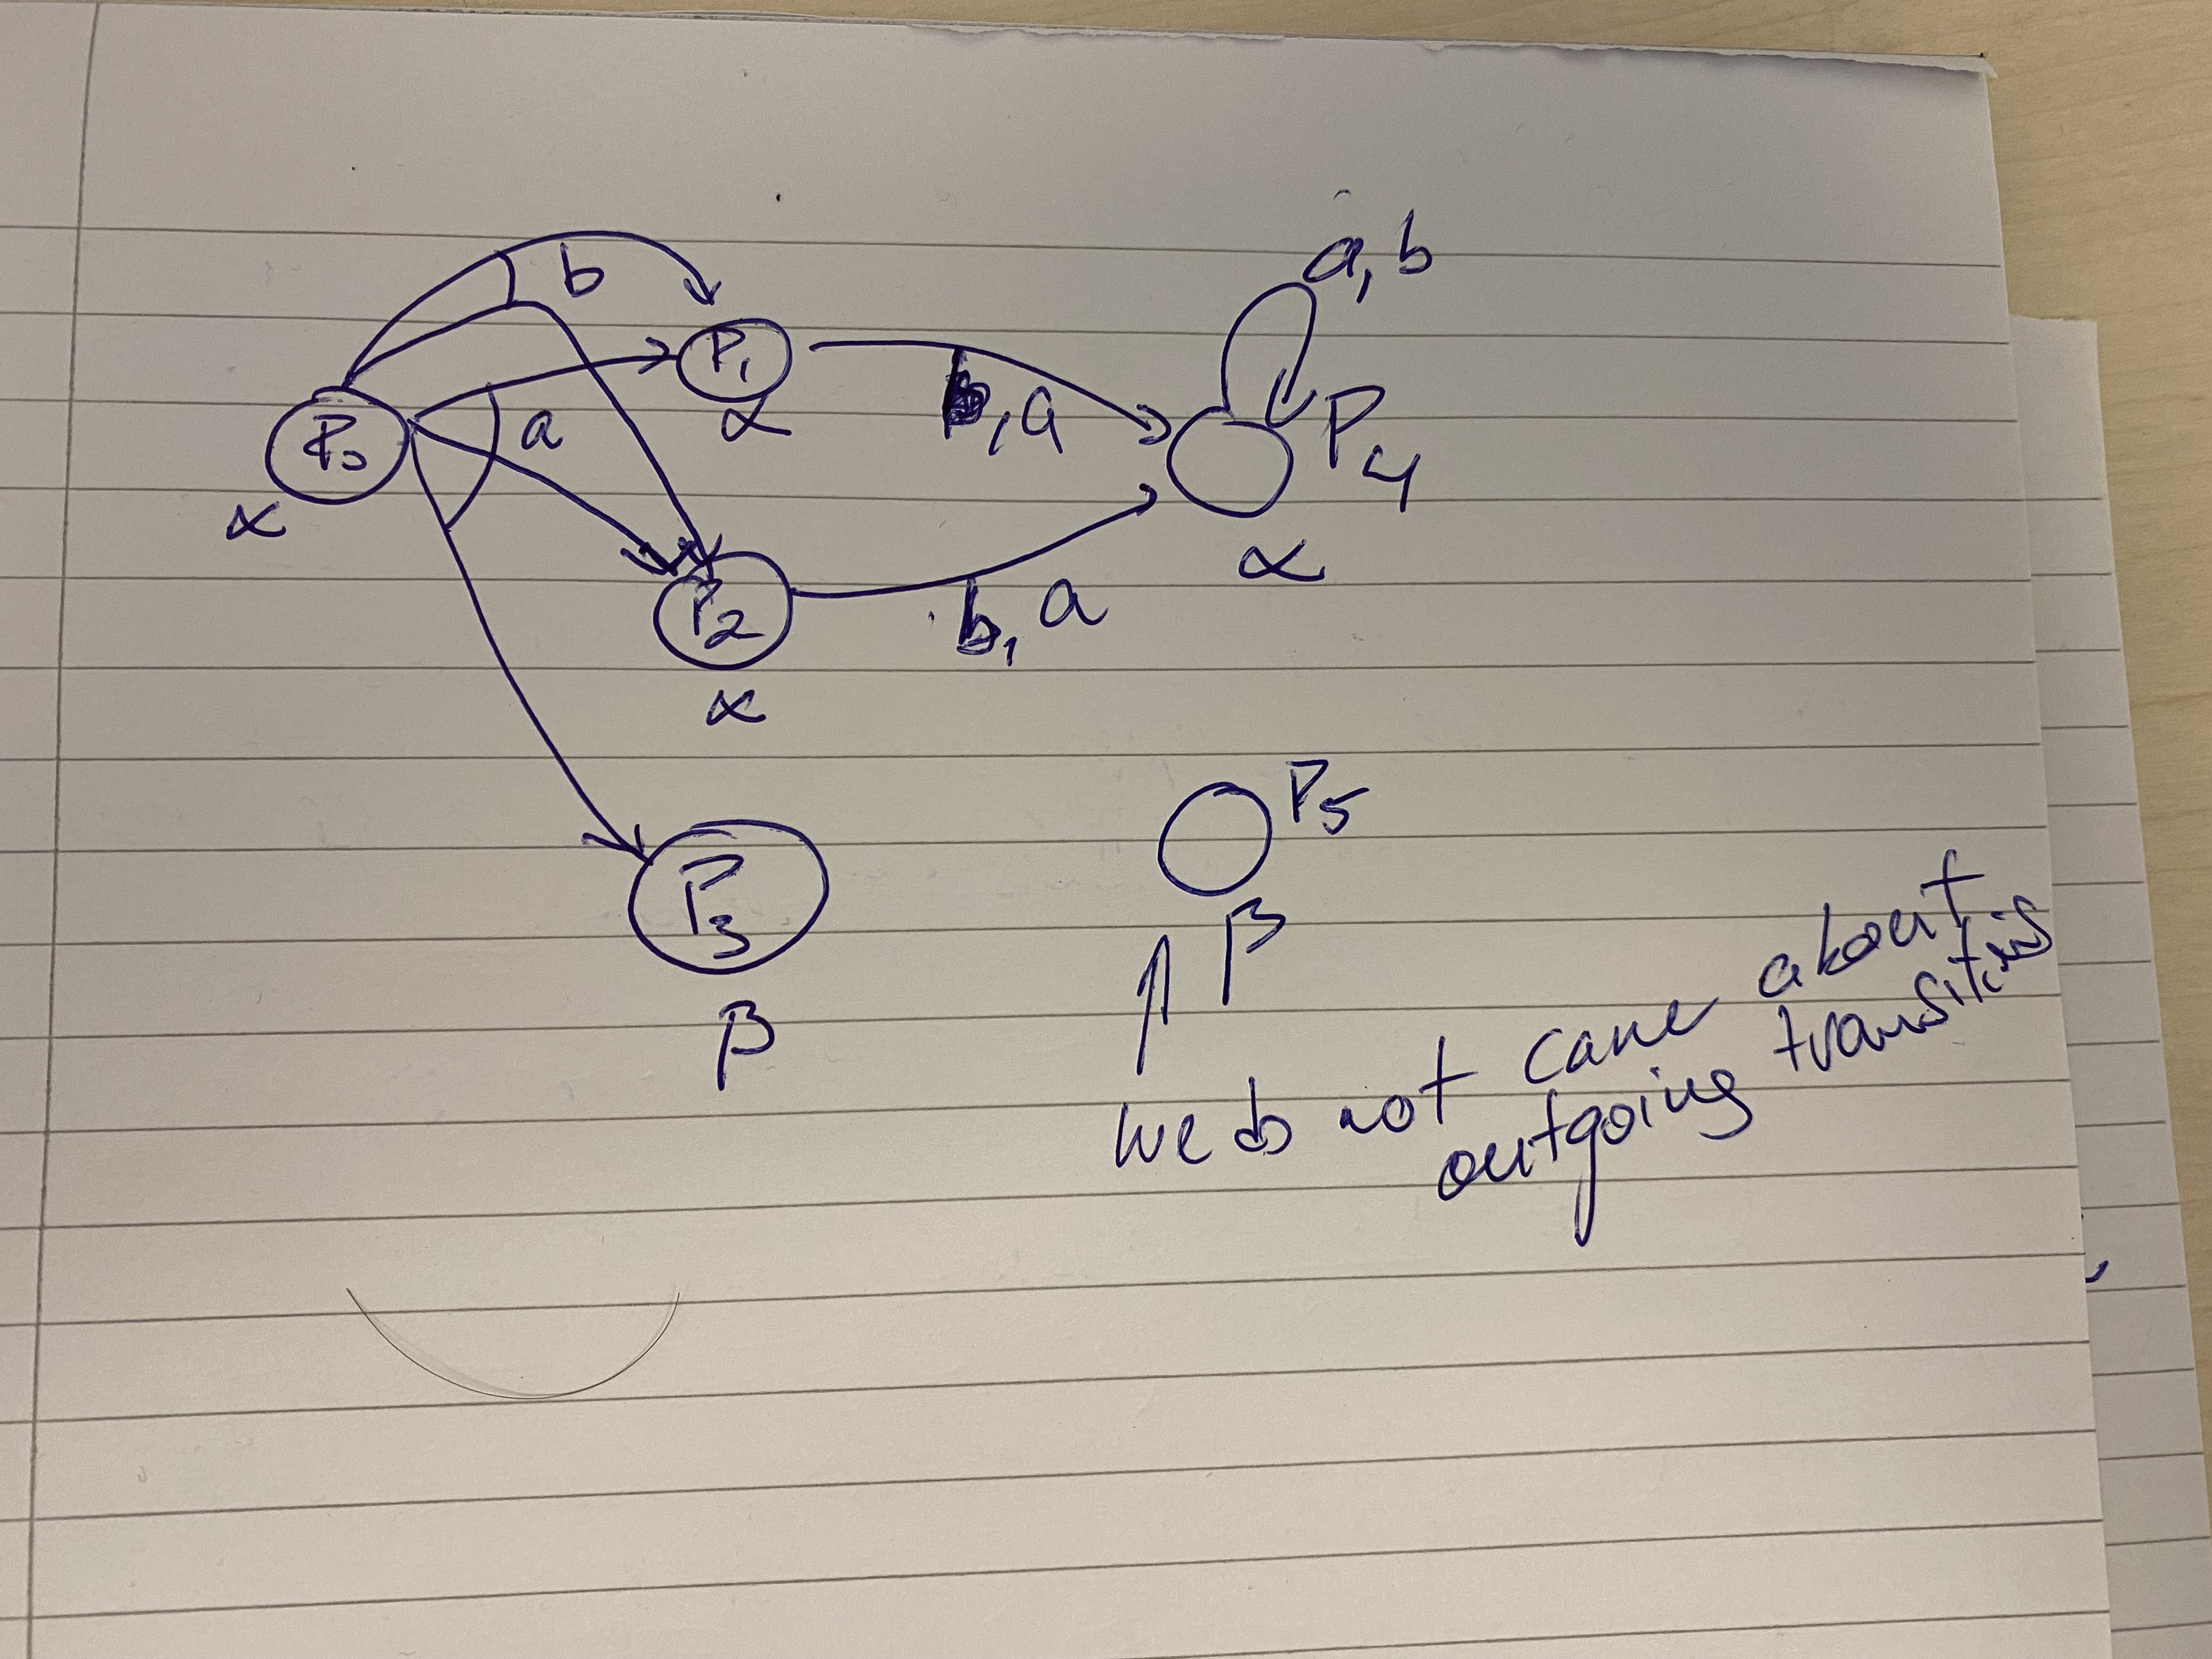}
    \caption{Sketch of the generated abstraction}
    \label{fig:my_label}
\end{figure}

Consider the following temporal property $\varphi = ``\text{ always $\alpha$ in the first 3 steps }''$ and notice that action $b$ is a valid action in the discrete model. However, despite the fact that the above abstraction satisfies the PAC-simulation notion as described in \cite{DSA:21}, we cannot refine the action $b$ into a valid action for the original system. In fact, the property $\varphi$ does not hold in the original system, thus providing a counterexample for the results in \cite{DSA:21}.
