# Supplementary material for: Data-driven memory-dependent abstractions of dynamical systems
Source: arXiv:2212.01926 source file (2022-12-04)
Supplement: Supplementary file 2 [file General_idea.tex]

\section{General Idea -- Inspired by the Google doc and internal discussions}
\label{sec:GeneralIdea}

Our goal is to produce stochastic abstractions for deterministic dynamical systems by means of a very coarse partition and uniformly sampling points in each element of the partition. The hope is that this will lead to smaller abstractions, and will possibly enable us to prove theoretical results relating the the original systems and its Markovian abstraction. Current results rely on the notion of incremental stability, which may be too restrictive and may require very fine partitions. 

The challenge of abstracting deterministic systems as stochastic models is that sometimes creating a Markovian abstraction -- by uniformly sampleing points in the partition and approximating the transition probability with empirical average -- may not be sound. we (namely, Raphael) is conjecturing that this problem may be mitigated through the use of memory and exploiting some notion of ``dissipation of information'', which is inspired by some literature in chaos theory and networked control systems.

After some internal discussions (and also having a look at the google docs, etc), we have came up with the following questions:

\begin{itemize}
    \item[1.] How shoul we call this uncertainty in our abstraction? 
    
    \licio{Given our discussion in the past week, Alessandro suggested that we are trying to convert the error made during the discretization step of the continuous dynamics (which is a source of epistemic uncertainty) into transition probabilities of our discrete stochastic abstraction. In principle, we can reduce such a discretization error by refining the partition (possibly using some information theoretic tools, as suggested by Raphael) and this would translate into a more precise transition probability in the obtained Markov model. So, despite the fact of being probability distribution, our current understanding is that this is a source of epistemic error. Any comments on this?}
    \raphael{I think we are pretty much in line. I woud rather say that it is ' a representation of our epistemic uncertainty' rather than a 'source of'... I think it might be a good tool for \emph{estimating heuristically} our epistemic uncertainty: now we can sample trajectories, and analyse the behaviour of our probabilistic abstraction (the markov chain), and compare... more about this tomorrow} 
    \item[2.] Formalize and quantify how far away the behaviour of the abstraction
is from the initial system; There's some kind of entropy/Lyapunovn exponent there.

    Here are some thoughts about this question. Let's consider a (deterministic) discrete-time dynamical system given by 
        \[
            x_+ = f(x), \quad x(0) = x_0,
        \]
        for some initial condition $x_0 \in \mathbb{R}^n$. Assume there is a unique equilibrium point at the origin that is a saddle point, namely, trajectories whose starting at the x-axis converges to zero and those starting from the y-axis blow up to infinity. Suppose that there exists a continuous function $\phi: \mathbb{R}^n \mapsto \mathbb{R}$ whose level sets separates the states into two invariant regions: one for which trajectories starting on it converge to zero (e.g., by approaching the x-axis and then converging to zero), and other where trajectories blow up to infinity. Let $(Q_i)_{i \in \mathcal{I}}$ be a partition of the state space and suppose there is one of the $Q_i's$ that intersects both of these regions. In this case, if we sample uniformly for such a partition we may find trajectories with distinct behaviours as described previously. We now reason about two types of partitions.
        \vspace{0.2cm}
        
        The first type of partition has a diameter\footnote{I am informaly thinking of the diameter associated with a collection of sets $(Q_i)_{\mathcal{I}}$ as $\max_{i \in \mathcal{I}} \mathrm{diam}(Q_i)$.} larger than a critical value (say $\bar{\delta}$) such that the proportion of partition with such an ambiguous behavior is ``relatively  high''; and the other case is the opposite. Another important quantity that may be related to a complexity notion of our abstraction procedure is some sort of distance between the maximal empirical distance between the transitions induced by subsets of each element of the partition.
        \vspace{0.2cm}
        
        After a few thoughts using the example above (and also inspired a bit from what I have read on Tomar's thesis), here is how I think we could quantify the above intuition and connect this with what Raphael suggested in this question. For a given collection of sets $(Q_i)_{\mathcal{I}}$, a collection of possible samples $m$ and the above dynamical system, consider the quantity $\eta_m(Q,f)$ defined as 
        \[
            \eta_m(Q,f) = \frac{\max_{i \in \mathcal{I}} \sup_{A_1,A2 \subset Q_i} \mathrm{KL}(\mathbb{P}_{m}(A_1), \mathbb{P}_{m}(A_2))}{\log_2(\frac{1}{\rho})},
        \]
        where $\mathbb{P}_{m}(A_j)$, $j = 1,2$, is the induced discrete measure induced in the discrete state by initializing the dynamics in points in $A_j$, $j = 1, 2$,\RJ{I don t understand: discrete measure of what? of the state after some time T?} \LR{Yes. I meant this to mean the measure induced in the partition of the state space (this is the reason I was referring to a discrete-measure) by running the dynamics for $T$ time steps.} and $\mathrm{KL}$ is the KL divergence between two probabilities measures, and $\rho$ is the fraction of elements of the partition for which the inner supremum is different from zero, i.e., for which we have heterogenous dynamics in the partition.
        \raphael{didn t understand why we take this strange formula inverse of logrho} \licio{This may not be correct, but my intuition would be that the complexity of the dynamics-partition pair, in addition to involving some distance due to distinct behaviours inside each element of the partition -- basically, the numerator above --, should take into account the frequency in which this happens. For a very fine partition, one should expect $\rho$ to go to zero, thus forcing the complexity to be small. Admittedly, this is a bit hand-waiving and should definitely be formalised. We may want to come back to this discussion later, or maybe this does not make sense at all.} The numerator of the above quantity denotes the number of bits (averaged) to describe the distance between the probability measures induces by our sampling procedure and the denominator is equal to the number of bit to quantify the number of elements that are ``bad''. Notice that a good pair $(Q,f)$ is one for which the above quantity is small. 
        
        Possible theorems and expected results:
        \begin{itemize}
            \item There should be a critical value for the diameter (and the memory adopted) of the sets for which we can show that the entropy above is bounded. If this quantity is large enough for a reasonably large class of the systems, then our method may lead to reasonable approximations. Hence we need to prove a result looking like the following statement: ``Given a vector field, a diameter and memory (should we induce a graph on the collection of sets for this?) there exists a $\bar{\delta}$ for which the above entropy is bounded for all partition with diameter less than $\bar{\delta}$.''

            \item We should then relate the above notion with some distance on the paths generated by the original system and its abstraction. Here is how this connects with the question Raphael mentioned above. To this end, we should try to prove a result that looks like the follow: ``For every collection of subsets (possibly with a graph structure to indicate the memory requirement) whose diameter is less than the critical value we have that:
            \[
                \| \phi(t) - \bar{\phi}(t) \| \leq B e^{g(n_m(Q,f))}, \quad B > 0,
            \]
            and $\eta_m(Q,f)$ as above"           
        \end{itemize}
\raphael{didn't understand everything but indeed it probably makes sense: we compare the different probability distributions that we obtain from the SAME cell of the partition: if they are different it means that our partition is bad. What I had in mind was a bit different: first we build a model of our system, THEN we have a closed form formula of it's behavior, THEN we can empirically evaluate the difference between the model and the true system. I have no idea what is more clever right now. Maybe my approach is more practical? (how to you compute your formula?)}
\licio{Most certainly, yes. I am not sure how one would compute the quantity I have written above. The main reason why I wrote this equation was to  provide room for the thinking process and define what is important and what it is not in the problem. I liked the way you presented the overall approach in our meeting today:
\begin{itemize}
    \item Take a toy example. We chose the sturmion dynamics.
    \item Create abstraction using Monte carlo simulation
    \item Define a complexity notion (I have tried to reason about this bit in the above comment). Such a notion should definitely distinguish ``simple'' (like $\theta$ being rational in the Sturmion dynamics) and complex ($\theta$ irrational) dynamics;
    \item Define a way to measure the distance of the generated trajecties in the abstraction with respect to the original dynamics.

    \item Develop a data-driven approach to compute such a distance.
\end{itemize}}
    
\end{itemize}

\begin{itemize}
    \item Lastly, it would be nice to have samples guarantees that asserts how many samples we to approximate $\eta_m$ above with
            \[
                \eta(Q,f) = \frac{\max_i \sup_{A_1,A_2} \log_2 \{ \# \text{ number of possible partitions} \}}{\log_2(\frac{1}{\rho})}.
            \]
    Convergence in measure using the scenario approach? 
\end{itemize}
