# Supplementary material for: Data-driven memory-dependent abstractions of dynamical systems
Source: arXiv:2212.01926 source file (2022-12-04)
Supplement: Supplementary file 3 [file LiteratureReview.tex]

\section{Literature Review}

In this Section I will try to summarize the main ideas related to some related literature. This would be initially based on a list of papers that Andrea Peruffo sent me last week but my plan is to gradually extend these comments. From the list he sent me we could identify some of the main players (in no particular order) in this field:
\begin{itemize}
    \item Calin Belta -- Boston University
    \item Rupak Majumdar -- Max Planck Institute for Software Systems
    \item Frank Allgower -- Univeristy of Stuttgart
    \item Matthias Althoff -- TUM
    \item Raphael Jungers -- UCLouvain
    \item Sadegh Soudjani -- Newcastle University
    \item Majid Zamani -- University of Colorado Boulder
    \item Alessandro Abate -- University of Oxford
    \item Samuel Coogan -- Georgia Tech
    \item Aaron Ames -- Caltech
    \item Dimos Dimarogonas -- KTH
\end{itemize}

I will begin making some comments on a series of paper by Aaron Ames.

\subsection{Aaron Ames}

I will start by reviewing the main ideas in the papers \cite{AA22,AAA22,ADABA22}. A common idea is to sampling uniformly a initial condition to generate samples of trajectories of dynamical system. Let $(\Omega,\mathcal{F})$ be a measurable space and $\mathcal{P}(\Omega)$ be a collection of probability measures on $\Omega$. Consider the following dynamics
\begin{equation}
    x(k+1) = f(x(k),\omega(k)), \quad x_0 = x(0)
    \label{eq:DynamicalSystemAaron},
\end{equation}
where $\omega(k)$ is distributed according to a distribution $\mathbb{P}_k \in \mathcal{P}(\Omega)$.
Assume that we have $m$ independent samples from $x_0$ according to a distribution $\mu$ and let's denote by $S = \{ x_0(1), \ldots, x_0(m) \}$ the collection containing these samples. For each $x_0(i) \in S$ we associate a trajectory of length $M+1$, which we denote by $T(i) = \{ x_0(i), \dots, x_{M+1}(i)\}$.

\begin{itemize}
    \item Claim 1: Denote by $\mathbb{Q}_k \in \mathcal{P}(\mathbb{R}^n)$ the distribution of the random variable $x(k)$, obtaining by running the trajectory of \eqref{eq:DynamicalSystemAaron} for $k$ steps. Notice that $\mathbb{Q}_k$ is equal to
    \scriptsize
    \begin{equation}
        \mathbb{Q}_k\{ x \in A\} = \int_{\mathbb{R}^n} d\mu (x(0)) \int_{\prod_{j = 1}^{k-2} \Omega} \prod_{j = 1}^{k-2} d\mathbb{P}_j(w(j)) \int_{A} \underbrace{(f\circ f \circ \ldots \circ f)}_{k-1 \text{ times }}(x(0),w(0),\dots,w(k-1)) d\mathbb{P}(w(k-1)), 
        \label{eq:DistributionStateSpaceAaron}
    \end{equation}
    \normalsize
    where $\underbrace{(f\circ f \circ \ldots \circ f)}_{k-1 \text{ times }}$ gives us $x(k)$, obained after sampling the initial condition according to $\mu$ and then following the stochastic dynamics according to the distribution of the noise.
    
    \item Claim 2: For each $k \in \{0,\ldots,M+1\}$, we have that $\{x_k(i)\}_{i = 1}^m$ is a collection of independent samples from the distribution $\mathbb{Q}_k$ defined in \eqref{eq:DistributionStateSpaceAaron}. This is a very tedious mathematical proof --- omitted for brevity.
\end{itemize}

When I read these papers from the first time, I had an issue with Claim 2 above, so I was thinking that we are obtaining samples from a distribution that changes with time hence the scenario approach theory could not be applied. But, after some thoughts, I believe I was wrong and indeed this may be a nice way to generate samples independent samples from the distribution $\mathbb{Q}_k$ defined in\footnote{I am not fully convinced of this yet, since I was lazy to try out the ``tedious'' mathematical proof above. But let's assume that Claim 1 and Claim 2 are true (btw, do you have a reasoning on why this could be false?)} \eqref{eq:DistributionStateSpaceAaron}.

Paper \cite{AA22} performs a verification task. Assume we are given a barrier candidate $h:\mathbb{R}^n \mapsto \mathbb{R}$. Our task is to check whether the zero level set of this function is invariant under the dynamics in \eqref{eq:DynamicalSystemAaron} within $K$ time steps when the dynamics in \eqref{eq:DynamicalSystemAaron} is deterministic, which could be understood in our setting by letting\footnote{In other words, the distubance is a constant and the right-hand side on \eqref{eq:DynamicalSystemAaron} is only a function of $x$.} $\mathbb{P}_k = \mathbb{P} = \delta_{\bar{x}}$, for some $\bar{x} \in \mathbb{R}^n$. To make things clearer, let's denote by $\mathrm{Lev}_0(h) = h^{-1}(-\infty,0]$ the zero level set of $h$. A sufficient condition to assert this is to show that existence of a $\gamma \in (0,1)$ for which
\[
\gamma h(x_k) \geq  h(x_k^+), \text{ for all } x_0 \in \mathrm{Lev}_0(h), \text{ for all } k = 1, \ldots, K,
\]
where $x_k^+$ is a short notation for the next state of $x_k$ according to the dynamics in \eqref{eq:DynamicalSystemAaron}. Since we are sampling the initial state and according to Claim 2 above we obtain a collection of independent random variables, we may solve this verification problem by means of the scenario program given by
\begin{align}
    \minimize_{\gamma \in (0,1)} & \quad \gamma \nonumber \\
    \mathrm{subject~to} & \quad h(x_k^+(i)) \leq \gamma h(x_k(i)), \text{ for all } k = 1, \ldots, K, i = 1, \ldots, m.
    \label{eq:ScenarioProgramAaron1}
\end{align}

\licio{Here is some inconsistency, according to my understanding though!}

The interesting phenomenon is the fact that the distributions $\mathbb{Q}_k$ will be different, even though the dynamics are deterministic. So, we cannot simply claim the scenario approach results to equation \eqref{eq:ScenarioProgramAaron1}. A fix to this approach -- which has not been done in \cite{AA22} would be to solve $k$ different scenario programs and combine somehow (need to look into the details) the solution returned for each one of them.

The setting of both \cite{AAA22,ADABA22} is similar to one described above, however, in this case we deal with true stochastic system as described in \eqref{eq:DynamicalSystemAaron}. The motivation stems from the risk-averse stochastic control literature and can be motivated as follows. Let $(\Omega,\mathcal{A},\mathbb{P})$ be a measure space and $X: \Omega \mapsto \mathbb{R}$ be a real-valed random variable. The \textit{Value-at-risk} ($\mathrm{VaR}_X (\epsilon)$) of level $\epsilon$ is defined as
\[
\mathrm{VaR}_X(\epsilon) = \inf_{F_X(s) \geq 1-\epsilon} s, \quad F_X(s) = \mathbb{P}\{ \omega \in \Omega: X(\omega) \leq s \}.
\]
In fact, the value-at-risk for a random variable is the optimal solution of the chance-constrained problem given by
\begin{align}
    \minimize_{s} & \quad s \nonumber \\
    \mathrm{subject~to} & \quad \mathbb{P}\{ \omega \in \Omega: X(\omega) \leq s \} \geq 1-\epsilon,
    \label{eq:ValueAtRiskAaron}
\end{align}
which can be approximated by the scenario theory using standard techniques. They have then used this formulation to verify whether the trajectories of a dynamical system described as in \eqref{eq:DynamicalSystemAaron} satisfies a specification given by a value-at-risk (which can be seen as an atomic proposition of STL). In other words, using trajectories of the model, they try to find an upper bound for which
\[
\mathrm{VaR}_{x(k)}(\epsilon) \leq \zeta, \text{ for all } k = 1, \ldots, K,
\]
where $x_k$ is the trajectory generated by the stochastic dynamics given in \eqref{eq:DistributionStateSpaceAaron}. Details are omitted but one can argue that they fall in the same pitfall as in the Barrier certification above. The companion paper uses similar ideas to consider more general risk measures; I will not discuss this here but happy to discuss more if necessary.

\subsection{Majid Zamani}

Majid has had several interesting works in the topics of data-driven abstractions of dynamical systems and Barrier certificate-based controllers with formal guarantees \cite{JSZ20,JPZ20,SSZ:20,SLSZ21,ZZC22,ZZC22b}. Let me start with the paper \cite{JPZ20}, where the authors combine Gaussian regression and Barrier functions to the design of controllers that satisfy safety specifications. 

The main idea of \cite{JPZ20} is to use Gaussian regression to estimate some envelop that contains the true dynamics with some confidence level, and then try to design a Barrier function that is robust against any possible dynamic in the generated envelop. The paper considers the following dynamical system
\[
\dot{x} = f(x) + g(x)u, \quad x(0) = x_0,
\]
where $f:\mathbb{R}^n \mapsto \mathbb{R}^n$ is assumed to be unknown and $g(x):\mathbb{R}^n \mapsto \mathbb{R}^n$ is a known function. The controller design is split into two steps:
\begin{itemize}
    \item In the first step data is collected and an estimate for the function $f$ is obtained by means of Gaussian regression. More specifically, a collection of $S = \{ x_1, \ldots, x_m\}$ points is sampled uniformly from the domain of $f$ and a model for $f$, denoted by $\hat{f}$, is obtained. Due to properties of Gaussian regression that I am skipping, one is able to obtain a guarantee of the type
    \[
        \mathbb{P}^m\{ (x_1,\ldots,x_m) \in \mathbb{R}^{nm}: \sup_{x \in \mathbb{R}^n} \|f(x) - \hat{f}(x) \|_{\infty} \leq \epsilon \} \geq (1-\beta)^m,
    \]
    where $\epsilon$ is a quantity that depends on proeprties of the kernel and the mutual information between the collected samples and the value of the function $f$. 
    \item By establishing the previous inequality, we may reformulate the original control problem as one of designing a feedback controller for
    \[
        \dot{x} = \hat{f}(x) + \epsilon + g(x)u, 
    \]
    where $\epsilon$ is a bounded control input and introduces non-determinism in the original dynamics. This can be done by searching for a Barrier function that satisfies standard conditions (details are omitted here for brevity).
\end{itemize}

\subsection{Rupak Majumdar}

In the paper \cite{KMSSW22}, the authors leverage the scenario approach theory to compute an abstraction with a guaranteed growth bound with respect to the nominal model. Consider the pair of dynamical systems given by
\[
    x_+ = f(x,u) + w,~x(0) = x_0, \quad s_+ = T(s,a),~s(0) = s_0,
\]
where we have a possible transition in the discrete model whenever it leads to an admissible trajectory in the continuous model. In this paper, the transition are computed by performing reachability computation. For a given state-action pair in the discrete model $(s,a)$, we define the set of reachable set in the continuous model as
\[
    \mathcal{R}(s,a) = \{ x_+ \in f(x,a): x \in \phi_{\mathcal{X}}^{-1}(s) \},
\]
where the discrete action are taken to be a discretization of the continuous dynamics, so the notation $f(x,a)$ is well-defined. The main idea in \cite{KMSSW22} is to use the scenario approach theory to compute, with high-probability, an envelop that contains all possible trajectories of the continuous dynamics (over-approximating the reachable sets). To this end, the authors tap into the result in the paper by Peyman to generate a feasible solution to a robust optimisation problem using a scenario program. In principle, I found the way they are employing the scenario approach to be correct, as they generate samples in the format $(x,u,x_+)$, and not by recording system trajectories. trajectories of the system.
where the discrete action are taken to be a discretization of the continuous dynamics, so the notation $f(x,a)$ is well-defined. The main idea in \cite{KMSSW22} is to use the scenario approach theory to compute, with high-probability, an envelop that contains all possible trajectories of the continuous dynamics (over-approximating the reachable sets). To this end, the authors tap into the result in the paper by Peyman to generate a feasible solution to a robust optimisation problem using a scenario program. In principle, I found the way they are employing the scenario approach to be correct, as they generate samples in the format $(x,u,x_+)$, and not by recording system trajectories.

In \cite{majumdar2020abstraction}, the authors focus on output-based control systems. They propose an adaptation of the notion of feedback refinement relation to this specific setting, and formalize the construction of an abstraction-based controller relying on the history of outputs. Even though in a different context (output-based control), their technique bears similarity to ours, in that past memory is used in order to store the previous observations, and the partition of the state-space according to the various possible observations is achieved.  In our approach, we use the same type of mathematical objects for the purpose of building a \emph{data driven} abstraction, and to relax the notion of abstraction with a probabilistic approach. 

\subsection{Jan Lunze}

In \cite{LN01}, the authors indeed propose an abstraction based on monte carlo sampling, and build a Markov model according to the relative frequencies. However, (as far as I could check), they do not leverage the probabilistic behaviour of their model whatsoever; indeed the the concept they introduce only depend on the \emph{possibility} of transitions (that is, whether the probability is larger than zero or not), and not on the numerical values of the different probabilities (unless I missed something?). The authors are interested in analysis of quantized systems, so, even though there are similarities in terms of mathematical notions, the framework and the motivation are quite different.

\raphael{I don't understand why I couldn't edit library.bib? the ref is here:}

\licio{I am generating the bib file from Mendeley, so I am not sure why Overleaf does not allow us to modify it. I have this reference into my database and also created another bib file called ``otherbibs.bib''. In the future, you can just add the references you want in the ``otherbibs.bib'' file -- I hope you are able to edit it. We will merge all the references into a single file in the final version of the draft. Would this be ok?}

\subsection{Stefan Kiefer}

We need to check whether \cite{kiefer2021approximate} is relevant to this work.

\raphael{I'll check if we should have a look at {kiefer2021approximate}}
