# Supplementary material for: Data-driven memory-dependent abstractions of dynamical systems
Source: arXiv:2212.01926 source file (2022-12-04)
Supplement: Supplementary file 4 [file Problem_formulation.tex]

\section{A possible mathematical formulation of the approach}
\label{sec:probFormulation}

Consider a discrete-time dynamical system given by
\begin{equation}
    x_{k+1} = f(x_k), \quad x(0) = x_0, \quad x_0 \sim \mu,
    \label{eq:dynamics}
\end{equation}
where $\mu$ is a probability measure over states. Raphael is arguing -- and we all agreed with him -- that an intuitive way to abstract the system is to first partition the state space and then observe trajectories of a fixed size from \eqref{eq:dynamics}; only then we create a discrete model representation of the dynamics under the basis of the generated language.

Here is what I planning to add below:

\begin{itemize}
    \item A description of the sturmian dynamics, as Raphael described below. This will serve as our toy model to test ideas.

    \item I will try to connect the construction of the Markov Chain (or whatever we will decide to call this model -- relation with push-down automata?) with the push-forward measure induced by the flow of \eqref{eq:dynamics}.
    \item A road map on how we should approach the problem. Namely, how to define a metric to measure the quality of the generated abstraction? Could we possibly do this using  information theoretic concepts developed in the RL or stochastic process community?

    \item How can we compute the metric defined in the previous item heuristically?
\end{itemize}

\subsection{Sturmian dynamics: a simple toy example}
\raphael{I think we all are on the same page here so I skip for the moment: basically $$x_{k+1}=x_{k}+\theta \quad \mbox{mod} 2\pi.$$

And the abstraction has only two cells: $$ [0,\theta] \quad [\theta, 2 \pi] .$$

}

\subsection{A (bold) proposal for a new smart monte-carlo abstraction}
For the moment we just analyse autonomous systems. The goal is to add control later \RJ{and it might well be a nontrivial step}
Again it seems simpler to tackle discrete-time systems at first.

\begin{enumerate}
    \item \label{algo-step1} Fix a partition (e.g. classical coordinate-plane parallel partition)
    \item Sample points in each cell, simulate trajectories of length $M\in \mathbb N$ \RJ{I assume here that we have a blackbox system which we can simulate. One could imagine other situations in engineering where we could apply similar procedures} and compute a jump probability function (one for every cell). \RJ{we can probably use PAC-like bounds here}
    \item Based on this heuristic probability distributions, we can build a markov chain where nodes correspond to cells, and the probability distributions are the ones inferred at the previous steps. We note it $P_M.$
    \item Now, compute the probability distribution for length $M'>M.$\RJ{typically, this corresponds to the matrix product operation: $\tilde P_{2M}=P_M^2,$ or $\tilde P_{M+1}=P_1P_M,$ where $P_1$ the probability matrix of the markov chain of length one.} 
In parallel, one can reiterate the monte-carlo computations above, with a simulation length equal to $M',$ to obtain a second Markov chain $P_{M'}$
    \item We now have two markov chains to compare. One way is to compute their perron vector, and then we have two probability distributions, on which we can compute a distance (Waserstein, TV, KL)\RJ{this is probably not completely new, but there are interesting results to be unraveled about the link between the metric chosen and the guarantees on teh performance.} \raphael{'How can we compute the metric defined in the previous item heuristically?' was a question of Licio. Here is just a suggestion. Don't know if it's the best one of course; but again, there is room for theorems here (but again, the link between loss function and performance has certainly a big literature)}

    \item Based on the discrepancy between our two models, we should be able to evaluate the conservatism of our model wrt the desired objective. Depending on that, either
    \begin{itemize}
        \item refine the abstraction at the critical nodes (critical in terms of discrepancy between our two models), and go back to step \ref{algo-step1}
        \item go with that partition if the discrepancy is small
    \end{itemize}
\end{enumerate}

\raphael{we could do more fun stuff later: eg: given an amount of time left before we have to deliver the controller, optimize the number of samples we take before to reiterate one more step}
\raphael{I would like to clarify how different it is to refine the abstraction vs. increase the memory (in a non-symmetric way; that is, I can only store eg the last two cells if the last cell is 0, but I store the last 10 cells if the last cell is 1...). Somehow refining the abstraction is equivalent to increase memory, but I'd like a formal statement for this}

\subsection{Links with literature}

\subsubsection{literature to check more carefully}
\begin{itemize}
    \item Munos' paper: smart insights to refine abstraction
    \item loss functions in RL
\end{itemize}

\subsubsection{Contributions from us wrt literature}
\begin{itemize}

    \item a new efficient data-driven approach, which does not rely on growth-bound or other conservative approaches
    \item expose (and formalize) the markovian problem, related with discretization
    \item a smart refinement algorithm, based on insight on the dynamics given by information-theoretic, or say probability, tools. 
    \item ... ?
\end{itemize}

\subsection{Roadmap and action points}

\raphael{I'm happy to try to motivate Adrien; I just think we should objectivise first whether we have sufficient novelty (I'm pretty convinced of that; in particular if the the goal is of designing smart abstractions for efficient symbolic control;  but...). But I can also contact him rightaway if we want to move faster.}

\begin{itemize}
    \item compare with literature (in particular RL)
    \item ask Mykel K. if it rings a bell
    \item implement the heuristic to have a POC: the system automatically generates an abstraction in a smart way; compare with classical refined abstraction approaches
    \raphael{we could check an LTL formula that we know is true thanks to our good theoretical understanding of the system e.g. the system must always output at least three times '001' between two occurences of '0001'}
\end{itemize}
