# Supplementary material for: Data-driven memory-dependent abstractions of dynamical systems
Source: arXiv:2212.01926 source file (2022-12-04)
Supplement: Supplementary file 5 [file paper_structure.tex]

\section{Structure of a paper}

\subsection{Intro}

In this paper we propose a novel, iterative, Monte-Carlo approach to build smart abstractions for complex dynamical systems. The goal is to have a good qualitative representation of the dynamics via sampling, thus alleviating complex analytic calculus which classically derive exact, but conservative, guarantees on the local behaviour of the system. 

By sampling the trajectories, we obtain an estimation of the (noisy) behaviour of the system: when one samples a particular cell, and a particular control input, he or she does not always obtain the same output. 
A drawback of generating abstractions by Monte-Carlo sampling is that it introduces spurious noise: the abstraction of the system relying on a discretization of it, we are bound to cope with some epistemic uncertainty on our system. In order to represent this uncertainty, and subsequently to tame it, we propose to represent it as a \emph{pseudo-aleatoric} uncertainty, and we reinterpret our monte-carlo abstraction as a Markov Chain.\\ 
We propose an iterative procedure allowing to refine in an efficient way our abstraction, thus reducing the epistemic uncertainty, via the notion of \emph{memory.} As a first theoretical contribution, we show that when one increases the memory, the epistemic uncertainty (and thus the pseudo-aleatoric uncertainty of our abstraction) decreases.  We propose a method to estimate online the remaining epistemic uncertainty, leading to a stopping criterion when the abstraction is sufficiently refined. Our technique also allows to refine the abstraction in a smart way, by identifying automatically the sources of epistemic uncertainty (i.e. the cells to be refined). \\
As a second theoretical contribution \RJ{not sure if that's gonna be easy} we provide a \lq simulation theorem \rq which, given the online estimation of a bound on the remaining uncertainty, provides a guarantee of approximability of the trajectories of the true system by the trajectories in the monte-carlo abstraction.

\subsubsection{Links with literature}

\begin{itemize}
    \item Munos' paper: smart insights to refine abstraction
    \item loss functions in RL
\end{itemize}

\subsubsection{Contributions from us wrt literature}
\begin{itemize}

    \item a new efficient data-driven approach, which does not rely on growth-bound or other conservative approaches
    \item expose (and formalize) the markovian problem, related with discretization
    \item a smart refinement algorithm, based on insight on the dynamics given by information-theoretic, or say probability, tools. 
    \item ... ?
\end{itemize}

\subsubsection{Proofs of concepts}
\begin{itemize}
    \item we show that we have less spurious trajectories than regular abstraction
    \item we show that we have an empirical way of estimating the number of spurious traj
    \item we use probabilities to even reduce the 'measure' of spurious traj
\end{itemize}

\subsection{The general methodology}

We consider a discrete-time dynamical system given by
\begin{equation}
    x_{k+1} = f(x_k), \quad x(0) = x_0, \quad x_0 \sim \mu,
    \label{eq:dynamics}
\end{equation}
where $\mu$ is a probability measure over states.
For the moment we just analyse autonomous systems. The goal is to add control later.  
Again it seems simpler to tackle discrete-time systems at first.

\begin{example}
The \emph{sturmian dynamics:} We fix a memory M, build the Markov chain, then simulate for longer time ($M+1,$ or $2M?$) and observe that the probability distribution of the small Markov Chain is spurious. This suggests to iterate in the following way:
\end{example}

\begin{enumerate}
    \item \label{algo-step1} Fix a partition (e.g. classical coordinate-plane parallel partition)
    \item Sample points in each cell, simulate trajectories of length $M\in \mathbb N$  and compute a jump probability function (one for every cell). 
    \item Based on this heuristic probability distributions, we can build a Markov chain where nodes correspond to cells, and the probability distributions are the ones inferred at the previous steps. We denote it as $P_M.$
    \item Now, compute the probability distribution for length $M'>M.$\RJ{typically, this corresponds to the matrix product operation: $\tilde P_{2M}=P_M^2,$ or $\tilde P_{M+1}=P_1P_M,$ where $P_1$ the probability matrix of the Markov chain of length one.} 
In parallel, one can reiterate the Monte-Carlo computations above, with a simulation length equal to $M',$ to obtain a second Markov chain $P_{M'}$
    \item We now have two Markov chains to compare. One way is to compute their Perron vector, and then we have two probability distributions, on which we can compute a distance (Waserstein, TV, KL). We propose first the formula $$ \sup_{k} {|| P'^k -P^k ||_\infty} $$ or
    $$ \sup_{k} {|| P'^k -P^k ||_\infty/(2^{M})} $$ or
    $$ \sup_{k} {|| P'^k -P^k ||_\infty/(2^{M+k})}. $$
    \item Based on the discrepancy between our two models, we should be able to evaluate the conservatism of our model wrt the desired objective. Depending on that, either
    \begin{itemize}
        \item refine the abstraction at the critical nodes (critical in terms of discrepancy between our two models), OR increase the memory $M,$ and go back to step \ref{algo-step1}
        \item go with that partition if the discrepancy is small
    \end{itemize}
\end{enumerate}

\begin{example}
First experiment: we compute the distance for increasing M and show that the distance goes to zero.

EDIT: for every $M$, we compute the $M$-memory model, and we lift the $M-1$ earlier models so that they are all comparable. That is, for every $M'<M,$ we take the $M-M'$-memory lift of the $M'$-memory model.
\end{example}

\begin{example}

Second experiment: we compare with a classical way of building an abstraction: we cut the circle in $M+1$ parts, and 
\begin{itemize}
    \item we build the Markov chain from this partition, and show that the distance is larger
    \item we use both our partitions in order to build a simulation. None of them will be a true bi-simulation of the concrete model, however, we show that we are much closer to a bisimulation than the 'stupid' discretization.
\end{itemize}
\end{example}

\begin{example}
The sturmian dynamics continued. We observe the evolution of the distance between the two Markov Chains when M increases, and we show that this distance decreases. Then, we successively refine the abstraction depending on the memory; that is, for a particular memory $M,$ we partition the state space according to the labels of length $M.$ We try to certify some LTL specification (e.g. there is never more than 3 zeros in a row) and we show that it allows for a more efficient way of verifying it.

This gives us a Proof of Concept.
\end{example}

\begin{example}
show that the monte carlo approach allows to construct a smart discretization of the system.
\end{example}

\subsection{Theoretical results}
In the first theorem, we show that for some measure function of the epistemic uncertainty, the function decreases when $M$ increases

For this we need to define unambiguously a notion of distance between the two MArkov chains. \RJ{I suggest this one to start with but I am not sure at all that the theorem is true!}

\begin{definition}
Given two Markov chains on the same set of nodes, we define $\pi,\pi'$ their perron vector. Then we define a probability distribution on the edges of these Markov chain: for any edge $e=(p,q),$ the probability $P(e):= \pi_p M_{p,q}.$
\end{definition}
\begin{definition}
Given two Markov chains on the same set of nodes, we define the \emph{Waserstein} (resp. \emph{KL, xxx}) distance between the two Markov chains the corresponding distance between the probability distributions on their edges, as defined above.
\end{definition}

\begin{theorem}
Consider a dynamical system as defined above, and our procedure of Monte-Carlo abstraction. When $M$ increases, the distance between the MArkov Chains with memory $M$ and $M+1$ decreases.
\end{theorem}

A second result would guarantee that our abstraction provides a sufficiently reliable symbolic model of reality, depending on the evaluated distance between the Markov chains.

\begin{theorem}
Consider a dynamical system as defined above, and our procedure of Monte-Carlo abstraction.Suppose that for some $M,$ the distance between the Monte-carlo abstraction of length $M+1$ and the MArkov chain obtained from the Monte-carlo abstraction of length $M$ is smaller than $\epsilon.$ Then, the the Monte-carlo abstraction of length $M$ is an $(\epsilon, \delta,XXX)$-abstraction of the system.
\end{theorem}
Needless to say one needs to define an $(\epsilon, \delta,XXX)$-abstraction of the system. But it's just to convey ideas at this point.

\raphael{All the above could be derived in the format where we do not put probabilities, but simply make an alternating simulation for worst-case controllability; or even simpler: a simple simulation for safety or reachability analysis; that is, no probabilities and no control. finally we could also, as said above, add control to the above setting, and we would have a MArkov Decision Process. }
