# Supplementary material for: Data-driven memory-dependent abstractions of dynamical systems
Source: arXiv:2212.01926 source file (2022-12-04)
Supplement: Supplementary file 6 [file ThoughtsMondayDiscussion.tex]

\section{Some thoughts}
\label{sec-thoughts}

sjhsdkj
