# Supplementary material for: Data-driven memory-dependent abstractions of dynamical systems
Source: arXiv:2212.01926 source file (2022-12-04)
Supplement: Supplementary file 7 [file questions.tex]

\section{Precise questions}
\label{sec:Questions}

\begin{itemize}
    \item Can we formalize the difference between our approach and others (say the AAAI approach) in terms of backwards reasoning for us, while the others are forward reasoning (cfr. AA's suggestion)
    
    \item More generally, how do we compare with other people's work?
    \item Intrinsically, memory is equivalent to refining partitions, but in practice, it's not the same action. Which one should we do and when? Idea: once the right memory is reached, the sampling provides us with a tentative partition corresponding to the sampled memory-traces, and we can perhaps make an a posteriori verification of this.
    
\end{itemize}
